# Supplementary material for: Diverse, Distinct, and Densely Packed DNA Droplets
Source: arXiv:2508.18574 source file (2025-08-26)
Supplement: Supplementary file 1 [file SI.pdf]

# Supplemental Material: Diverse, Distinct, and Densely Packed DNA Droplets

Aria S. Chaderjian,<sup>1</sup> Sam Wilken,<sup>1,2</sup> and Omar A. Saleh<sup>1,2</sup>

<sup>1</sup>*Physics Department, University of California,  
Santa Barbara, California 93106, USA*

<sup>2</sup>*Materials Department, University of California,  
Santa Barbara, California 93106, USA*

(Dated: August 25, 2025)

Movie S1. Time series of the quenched 7-NS system at late times, where there is sufficient free area for droplets to diffuse. Time after reaching 25°C is shown in hour:minute format. This is the same field of view shown in Fig. 5A.

Movie S2. Time series of the quenched 7-NS system at early times, where droplets are packed closely and exhibit dynamic heterogeneity. Time after reaching 25°C is shown in hour:minute format. This is the same field of view shown in Fig. 5A.

Movie S3. Time series of the quenched 7-NS system at early times, cropped to highlight an example of a coalescence event leading to other coalescence events. Time after reaching 25°C is shown in hour:minute format.

## **S1. UNCERTAINTY IN THE THERMODYNAMIC PARAMETERS GOVERNING DNA DUPLEX FORMATION**

Here we support the claim in the main text that the DNA thermodynamics dataset of SantaLucia and Hicks (‘SH’) [1] indicates an uncertainty in knowledge of the free energy of hybridization,  $\Delta G$ , of about 0.4 kcal/mol. The SH paper focuses on finding sequence-specific nearest-neighbor thermodynamic parameters that correctly predict the melting temperature,  $T_m$ , of duplex formation. The key relation is Eq. 3 of the SH paper, which (slightly adapted) reads:

$$T_m = \frac{1000\Delta H^\circ}{\Delta S^\circ + R \ln(C_T)} \tag{S1}$$

where  $\Delta H^\circ$  and  $\Delta S^\circ$  are, respectively, the temperature-independent enthalpy and entropy of hybridization of a full oligomer;  $R = 1.9872$  cal/K mol is the gas constant; and  $C_T$  is the total concentration of oligos in Molar. Note we have chosen a version of the equation that applies to self-complementary (palindromic) oligos, as is appropriate for our system. The factor of 1000 accounts for SH’s choice to tabulate  $\Delta H^\circ$  values in units of kcal/mol, while  $R$  and  $\Delta S^\circ$  are both used in units of cal/K mol. With these choices,  $T_m$  is given in absolute temperature (K).

Applying error-propagation to Eq. S1 gives the relation of uncertainty in  $T_m$ ,  $\sigma_T$ , to that

of the enthalpy and entropy,  $\sigma_H$  and  $\sigma_S$ :

$$\left(\frac{\sigma_T}{T_m}\right)^2 = \left(\frac{\sigma_H}{\Delta H^\circ}\right)^2 + \left(\frac{\sigma_S}{\Delta S^\circ + R \ln(C_T)}\right)^2 \quad (\text{S2})$$

For relevant concentrations of  $\approx 10 \mu\text{M}$ , we have  $R \ln(C_T) \approx -20 \text{ cal/K mol}$ , much smaller than the magnitude of  $\Delta S^\circ \approx -150 \text{ cal/K mol}$  that is relevant for the specific oligos used here. Thus, to good approximation, the  $R \ln(C_T)$  term in Eq. S2 can be ignored, and the relation reduces to a simple quadrature relation of relative uncertainties.

If we then assume that the relative uncertainty in knowledge of enthalpy and entropy are the same,  $\sigma_H/\Delta H^\circ = \sigma_S/\Delta S^\circ \equiv \bar{\sigma}$ , we find

$$\bar{\sigma} = \frac{\sigma_T}{T_m \sqrt{2}} \quad (\text{S3})$$

SH indicates that the standard deviation between their model and experiment is 2.3 K; taking this to be  $\sigma_T$ , then using the SH model to calculate  $T_m$  at  $C_T = 12 \mu\text{M}$  (i.e. the sticky end concentration for 3  $\mu\text{M}$  of 4-armed NSs), we find  $\bar{\sigma} \approx 0.006$ , i.e. there is a 0.6% uncertainty in both  $\Delta H^\circ$  and  $\Delta S^\circ$ . Using this uncertainty, propagated through the relation  $\Delta G = \Delta H^\circ - T \Delta S^\circ$ , results in an absolute error estimate of around 0.4 kcal/mol in the value of  $\Delta G$ , as utilized in the main text.

## S2. DNA SEQUENCES

| Name                  | Sequence                                                                     |
|-----------------------|------------------------------------------------------------------------------|
| 1/4-3'Cy5oh1gTc1jTT   | CCA ATT CGA CGA TTA GAC CGT TCT GGA TTC TCA GAA GTA GGG TGG GCC C/3Cy5sp/    |
| 1/4-3'oh1gTc1jTT      | CCA ATT CGA CGA TTA GAC CGT TCT GGA TTC TCA GAA GTA GGG TGG GCC C            |
| 2/4-3'oh1gTc1jTT      | CCC TAC TTC TGA GAA TCC AGT TCG ATC ATA AGG CTG GCC GTC TGG GCC C            |
| 3/4-3'oh1gTc1jTT      | GAC GGC CAG CCT TAT GAT CGT TCG TAA CGT GAG GTG ATA GTC TGG GCC C            |
| 4/4-3'oh1gTc1jTT      | GAC TAT CAC CTC ACG TTA CGT TCG GTC TAA TCG TCG AAT TGG TGG GCC C            |
| 1/4-3'Cy5oh2gTc2jTT   | CCC ATC GGC TTG GTT GCT CTT GTT CGT GCT TAG CGG AAA GTC TCA TGA G/3Cy5sp/    |
| 1/4-3'oh2gTc2jTT      | CCC ATC GGC TTG GTT GCT CTT GTT CGT GCT TAG CGG AAA GTC TCA TGA G            |
| 2/4-3'oh2gTc2jTT      | CTT TCC GCT AAG CAC GAA CTT GAT CTA TAA AGT GAA ACA CTC TCA TGA G            |
| 3/4-3'oh2gTc2jTT      | GTG TTT CAC TTT ATA GAT CTT CCT ACT CAG ATG CGG GCG GTC TCA TGA G            |
| 4/4-3'oh2gTc2jTT      | CCG CCC GCA TCT GAG TAG GTT GAG CAA CCA AGC CGA TGG GTC TCA TGA G            |
| 1/4-3'Cy5oh3gTc3jTT   | GTA GCT TGT GTA TAA ATT CTT CAA TTA ACA GAA GAC CCG GTT TTG CAA A/3Cy5sp/    |
| 1/4-3'oh3gTc3jTT      | GTA GCT TGT GTA TAA ATT CTT CAA TTA ACA GAA GAC CCG GTT TTG CAA A            |
| 2/4-3'oh3gTc3jTT      | CCG GGT CTT CTG TTA ATT GTT CCC ACT CAT AAT CGG CCT GTT TTG CAA A            |
| 3/4-3'oh3gTc3jTT      | CAG GCC GAT TAT GAG TGG GTT GAG GAA GCC CAT ACG CTA GTT TTG CAA A            |
| 4/4-3'oh3gTc3jTT      | CTA GCG TAT GGG CTT CCT CTT GAA TTT ATA CAC AAG CTA CTT TTG CAA A            |
| 1/4-5'Cy3oh4gTc4jTT   | /5Cy3/ ACG CGT TCC GAC GTG CCG GAG AAG CAG TTC TGG TGT CAC ACC GAA GGC G     |
| 1/4-5'oh4gTc4jTT      | ACG CGT TCC GAC GTG CCG GAG AAG CAG TTC TGG TGT CAC ACC GAA GGC G            |
| 2/4-5'oh4gTc4jTT      | ACG CGT TCG CCT TCG GTG TGA CAC CAG TTG GTA AAG GTG AGC GAG ACTC             |
| 3/4-5'oh4gTc4jTT      | ACG CGT TGA GTC TCG CTC ACC TTT ACC TTG CTT ATT CGT CTG CAT CAA G            |
| 4/4-5'oh4gTc4jTT      | ACG CGT TCT TGA TGC AGA CGA ATA AGC TTC TGC TTC TCC GGC ACG TCG G            |
| 1/4-5'Cy3oh5gTc5jTT   | /5Cy3/ GAT CGA TCT CTC CTG CCA AGT AAG ACG CTT GTC GGA GTA CAC TTA TGT G     |
| 1/4-5'oh5gTc5jTT      | GAT CGA TCT CTC CTG CCA AGT AAG ACG CTT GTC GGA GTA CAC TTA TGT G            |
| 2/4-5'oh5gTc5jTT      | GAT CGA TCT CAC ATA AGT GTA CTC CGA CTT CGC TGT TAT CTG CTC TCG G            |
| 3/4-5'oh5gTc5jTT      | GAT CGA TCT CCG AGA GCA GAT AAC AGC GTT CAT AGG CCT TCA ACC AGG G            |
| 4/4-5'oh5gTc5jTT      | GAT CGA TCT CCC TGG TTG AAG GCC TAT GTT GCG TCT TAC TTG GCA GGA G            |
| 1/4-5'Cy3oh6gTc6jTT   | /5Cy3/ CCT TAA GGT CGT TGA CAT ATC CCG CTC GTT CTT TAA TGA TCA CGT AGG C     |
| 1/4-5'oh6gTc6jTT      | CCT TAA GGT CGT TGA CAT ATC CCG CTC GTT CTT TAA TGA TCA CGT AGG C            |
| 2/4-5'oh6gTc6jTT      | CCT TAA GGT GCC TAC GTG ATC ATT AAA GTT GGG CGC ACG AGA CCT ATC G            |
| 3/4-5'oh6gTc6jTT      | CCT TAA GGT CGA TAG GTC TCG TGC GCC CTT GAC TGG ACC CAA ACG CCG G            |
| 4/4-5'oh6gTc6jTT      | CCT TAA GGT CCG GCG TTT GGG TCC AGT CTT CGA GCG GGA TAT GTC AAC G            |
| 1/4-3'At488oh7gTc7jTT | GGA GTC TAC TAC CGA CGG GTT GTG TGG GCG TGC CAG TGG CTC TAG CTA G/3ATTO488N/ |
| 1/4-3'oh7gTc7jTT      | GGA GTC TAC TAC CGA CGG GTT GTG TGG GCG TGC CAG TGG CTC TAG CTA G            |
| 2/4-3'oh7gTc7jTT      | GCC ACT GGC ACG CCC ACA CTT CAT CGC ATT ACG GCC GAA CTC TAG CTA G            |
| 3/4-3'oh7gTc7jTT      | GTT CGG CCG TAA TGC GAT GTT CTG TCA CGT CCA CCA TTG CTC TAG CTA G            |
| 4/4-3'oh7gTc7jTT      | GCA ATG GTG GAC GTG ACA GTT CCC GTC GGT AGT AGA CTC CTC TAG CTA G            |
| 1/4-3'At488oh8gTc8jTT | GTA TCA GGC TCC GAT GCG CTT CAT ACT CTT CTT AAC AAC CTG GAA TTC C/3ATTO488N/ |
| 1/4-3'oh8gTc8jTT      | GTA TCA GGC TCC GAT GCG CTT CAT ACT CTT CTT AAC AAC CTG GAA TTC C            |
| 2/4-3'oh8gTc8jTT      | GGT TGT TAA GAA GAG TAT GTT CTG CCG CGC CTC GAG TCC CTG GAA TTC C            |
| 3/4-3'oh8gTc8jTT      | GGG ACT CGA GGC GCG GCA GTT CCG CCA TCC CTC CAT TTC GTG GAA TTC C            |
| 4/4-3'oh8gTc8jTT      | CGA AAT GGA GGG ATG GCG GTT GCG CAT CGG AGC CTG ATA CTG GAA TTC C            |
| 1/4-3'At488oh9gTc9jTT | GCG TCT ACA GGT CGC TGG GTT GGA CGG ACG TAA GCA GCA CTC TGT ACA G/3ATTO488N/ |
| 1/4-3'oh9gTc9jTT      | GCG TCT ACA GGT CGC TGG GTT GGA CGG ACG TAA GCA GCA CTC TGT ACA G            |
| 2/4-3'oh9gTc9jTT      | GTG CTG CTT ACG TCC GTC CTT GAT CGG CGG GAC CCT TAG CTC TGT ACA G            |
| 3/4-3'oh9gTc9jTT      | GCT AAG GGT CCC GCC GAT CTT GTT TGG CAT CTT GGT GCC GTC TGT ACA G            |
| 4/4-3'oh9gTc9jTT      | CGG CAC CAA GAT GCC AAA CTT CCC AGC GAC CTG TAG ACG CTC TGT ACA G            |

TABLE S1. DNA sequences used in this work, written in triplets for legibility, and listed from 5' to 3'. The naming scheme is as follows: 'x/4' identifies the oligo among the 4 strands that comprise a given NS; 3' or 5' indicates the location of the sticky end (and, for fluorescently labeled strands, the location of the fluorophore); 'oh#' identifies the sticky end, with the number corresponding to NS numbers in the main text; 'gT' indicates that the unpaired base between the sticky end and the NS arm is a Thymine; 'c' identifies the internal (core) sequence, which always match the name of the sticky end; 'jTT' indicates two unpaired Thymine bases at the junction where the 4 arms of the NS come together.

### S3. SUPPLEMENTAL FIGURES

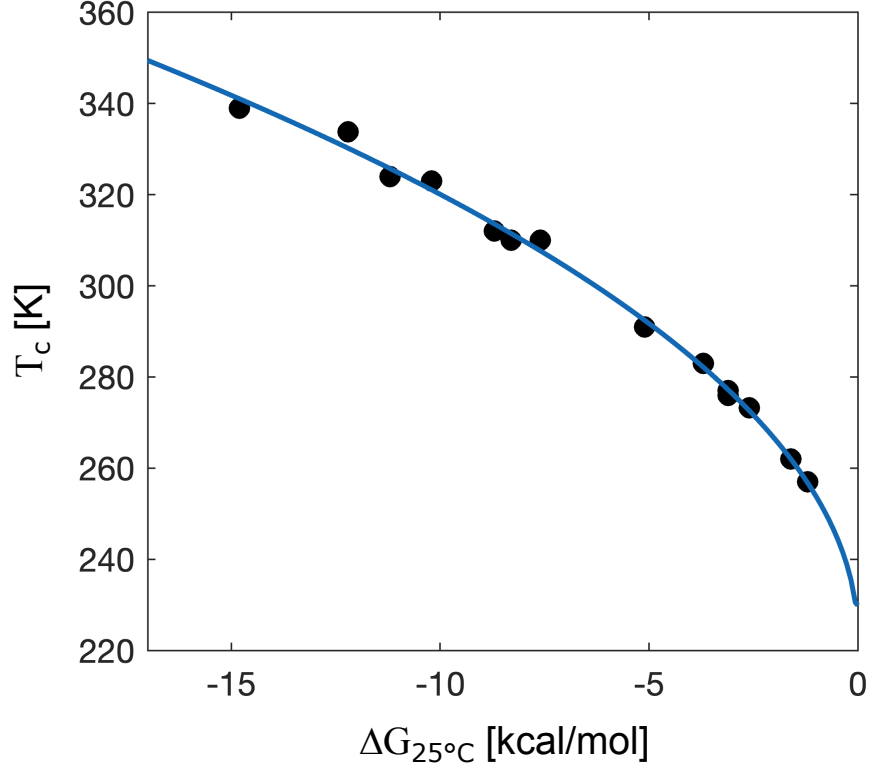

FIG. S1. Theoretically predicted critical temperature,  $T_c$ , plotted as a function of sticky end hybridization free energy  $\Delta G$  at  $25^\circ\text{C}$  as shown in Fig. 1D. The functional form of the free energy is evaluated by following Ref. [2]. It combines the Wertheim theory, which models NSs as hard sphere colloids with anisotropic sticky patches, with DNA hybridization thermodynamics.  $T_c$  is defined as the temperature at which the second and third derivatives of the free energy (with respect to density) are zero. The line shows that  $T_c$  is well predicted by a power-law functional form  $T_c(\Delta G) = 30|\Delta G|^{1/2} + 225$ , as found by two-parameter fitting. A subset of the points are shown.

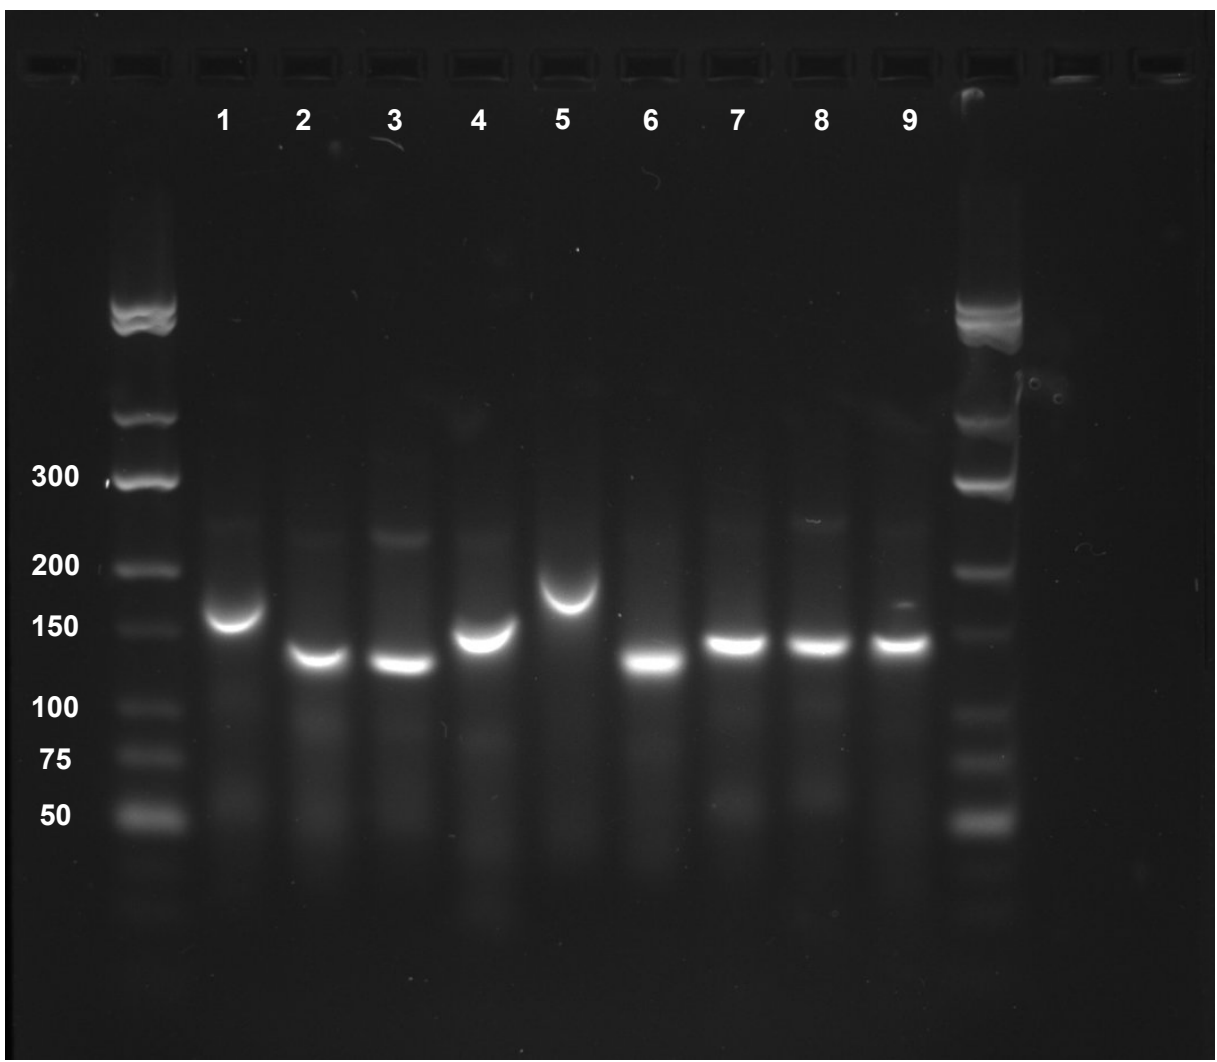

FIG. S2. Agarose gel electrophoresis of each annealed NS, confirming proper assembly. Lanes are numbered according to the NS number given in the main text. The reference ladder is numbered according to the length (in basepairs) of each band.

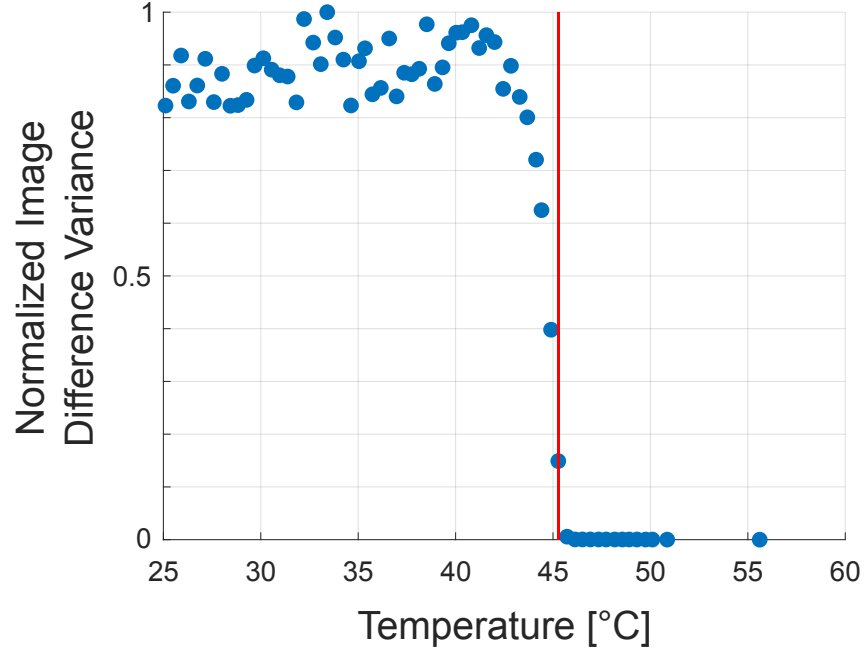

FIG. S3. Representative example of the procedure for estimating  $T_m$  from a temperature ramp. Image difference variance was calculated by computing the difference between subsequent images in the temperature ramp, in this case for NS1, and calculating the variance of that resultant image. Image difference variance significantly increases at  $T_m$  as droplets form. Image difference variance is normalized on the interval  $[0, 1]$ . The red line denotes  $T_m$  for this particular experiment, which is 45.3°C.

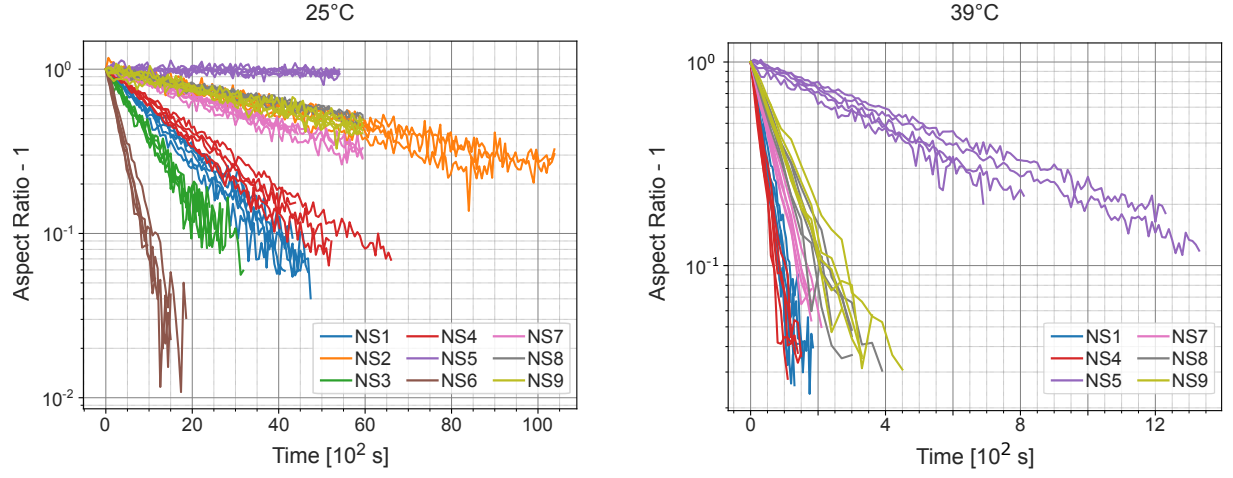

FIG. S4. Semi-log plots of the dynamics of the aspect ratio of coalescing droplets, confirming exponential relaxation in all cases. The 5 traces for each NS for each temperature reflect the data used for the creation of Fig. 2D. Here, each trace was normalized such that the initial value is 1.

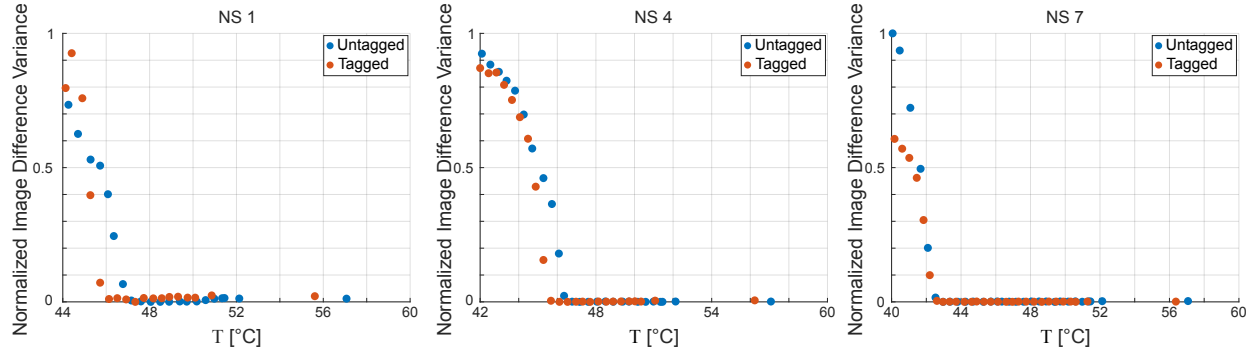

FIG. S5. Image difference variance plots for temperature ramps comparing fluorescently tagged and untagged NS mixtures, with tagged NS mixtures consistent with dye and percentage as indicated in main text for each NS (Fig. 3A). Altogether, these plots show that differences in dye and percentage of tagged particle are not responsible for the spread of  $T_m$  discussed in the main text (Fig. 2B). Image difference variance was normalized on the interval  $[0, 1]$ . For comparison, bright field images were used for both the tagged and untagged samples.

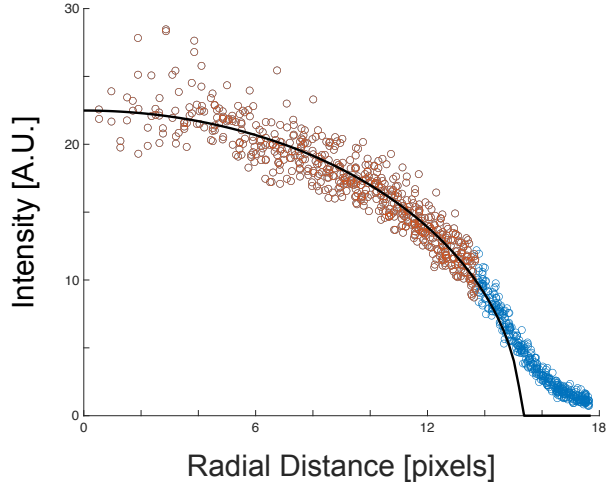

FIG. S6. Illustration of the method to measure droplet radius for the clustering analysis, showing a representative radial intensity profile of a droplet and the fit (black). Orange points indicate intensity values which were used for the fit, corresponding to pixels inside the droplet as determined by thresholding. 1 pixel =  $0.733 \mu\text{m}$ . Prior to fitting, images were processed by dividing by the homogeneous fluid image, where the darkfield value was subtracted from both the image and the homogeneous image. Droplet centroids and estimates of the radii were obtained from thresholding, as described in the Methods. The radial intensity profile inside the droplet was fit to the projection of a sphere onto 2-dimensions:  $I(x) = \int_{-\sqrt{R^2-x^2}}^{\sqrt{R^2-x^2}} b dz \Theta(R-x) = 2bR\sqrt{1-\left(\frac{x}{R}\right)^2}\Theta(R-x)$  where  $b$  is the constant intensity per unit height of each voxel,  $R$  is the droplet radius,  $x$  is the radial distance from the center, and  $\Theta(x)$  is the Heaviside function. Values for  $b$  were normalized for each fluorescent channel on the interval  $[0, 1]$ ; clusters in these normalized values,  $\bar{I}$ , enabled droplet classification (Fig. 3).

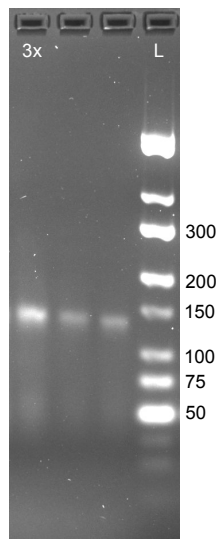

FIG. S7. Agarose gel electrophoresis was used to roughly estimate the concentration of NSs in the dilute solution of a phase separated sample containing all 9 NSs (untagged) at  $3\ \mu\text{M}$  each and 500 mM NaCl. The bands in the reference ladder are labeled by length in basepairs. The estimate was performed by comparing the intensity of the bands from the dilute solution to to the intensity of the bands in the ladder, and indicates the dilute solution contains  $\approx 0.4\ \mu\text{M}$  each NS. The image was brightened here for visibility. To obtain the dilute sample, a solution containing all 9 NSs (untagged) at  $3\ \mu\text{M}$  each and 500 mM NaCl was prepared, heated to  $55^\circ\text{C}$ , and subjected to the same thermal protocol as Fig. 3E (see Methods) while on a rotator. Upon reaching  $25^\circ\text{C}$ , the sample tube was held upright at  $25^\circ\text{C}$  for 6 hours to allow NS droplets to sediment to the bottom of the tube. The sample tube was centrifuged and the supernatant was extracted, diluted 3x, and loaded into the gel. The gel's background intensity value was subtracted from the image. The intensity of the 3x lane was compared to the intensity of the 100 basepair band, whose mass was provided by the supplier, allowing for the conversion of intensity to mass. The concentration of NSs in the dilute solution was thus obtained and divided by 9, assuming each NS contributed equally to the dilute solution concentration.

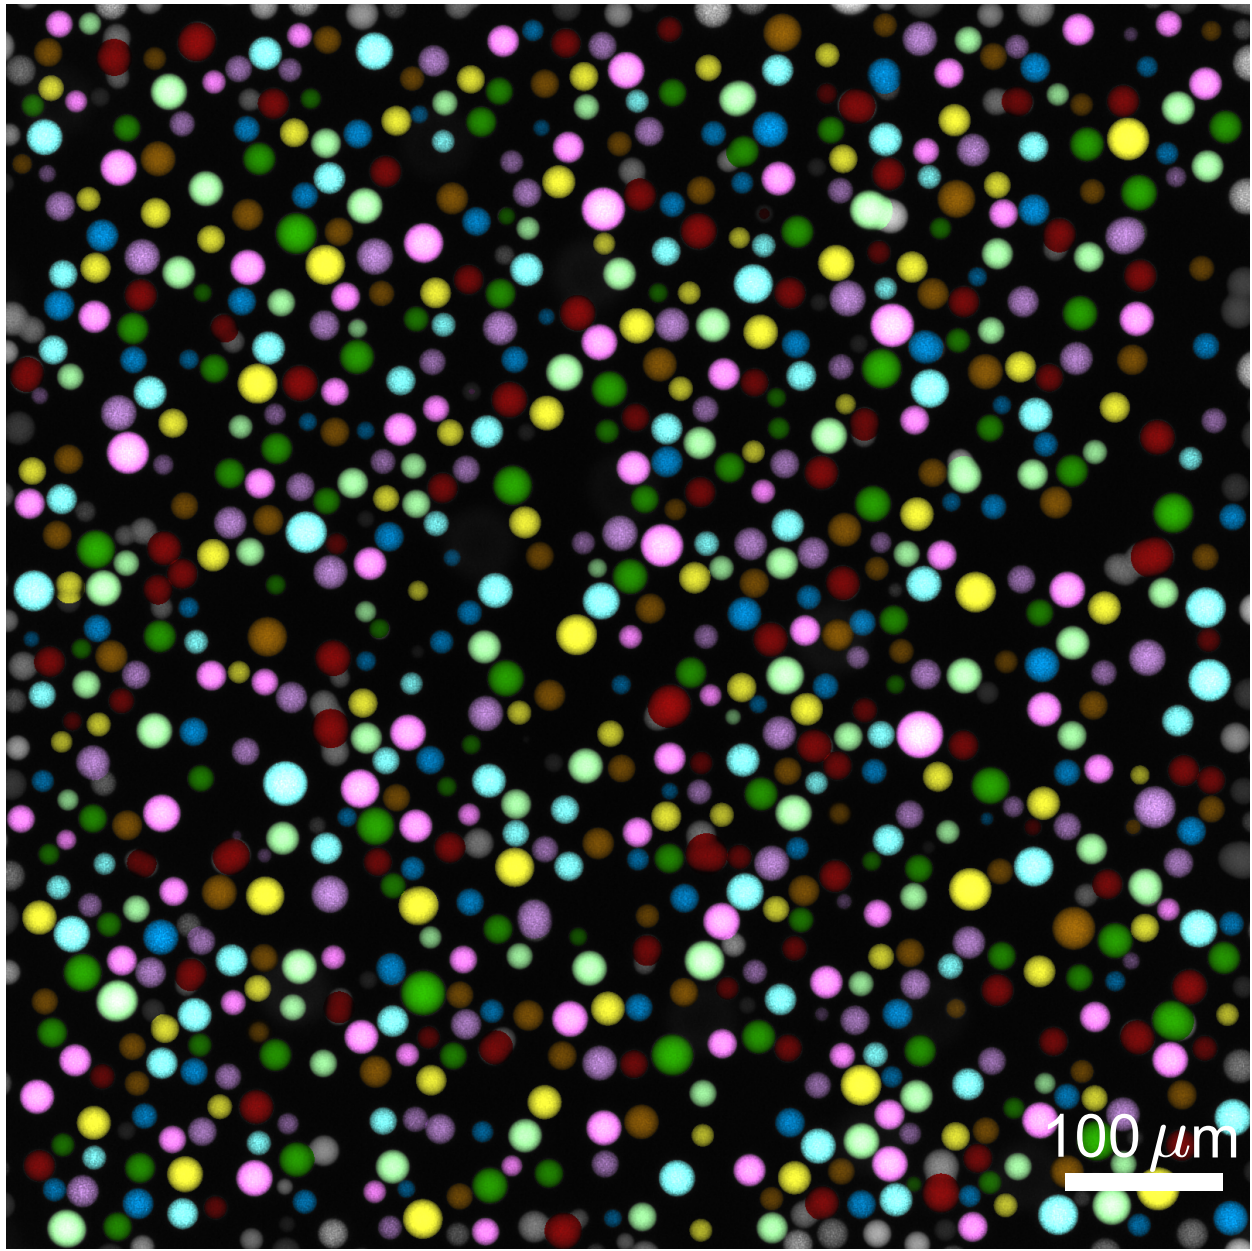

FIG. S8. Full size, false-colored image of 9 droplet phases associated with Fig. 3D in the main text. Most droplets that were not colored are undergoing a coalescence event.

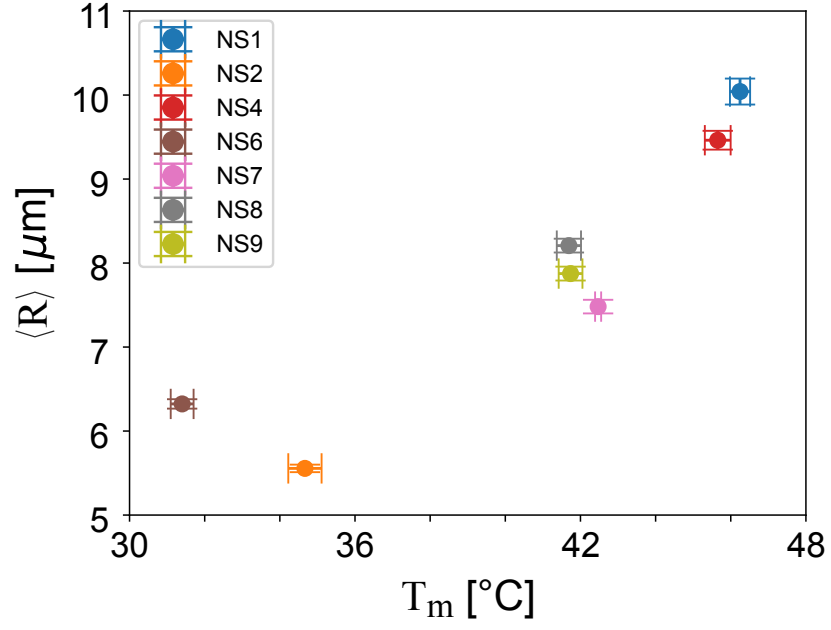

FIG. S9. Mean droplet radius vs. mean  $T_m$  for each of the 7 phases 4 hours after performing the temperature ramp corresponding to main text Fig. 4A, calculated from the full size image associated with the cropped image shown in the main text. Error bars reflect the SEM.

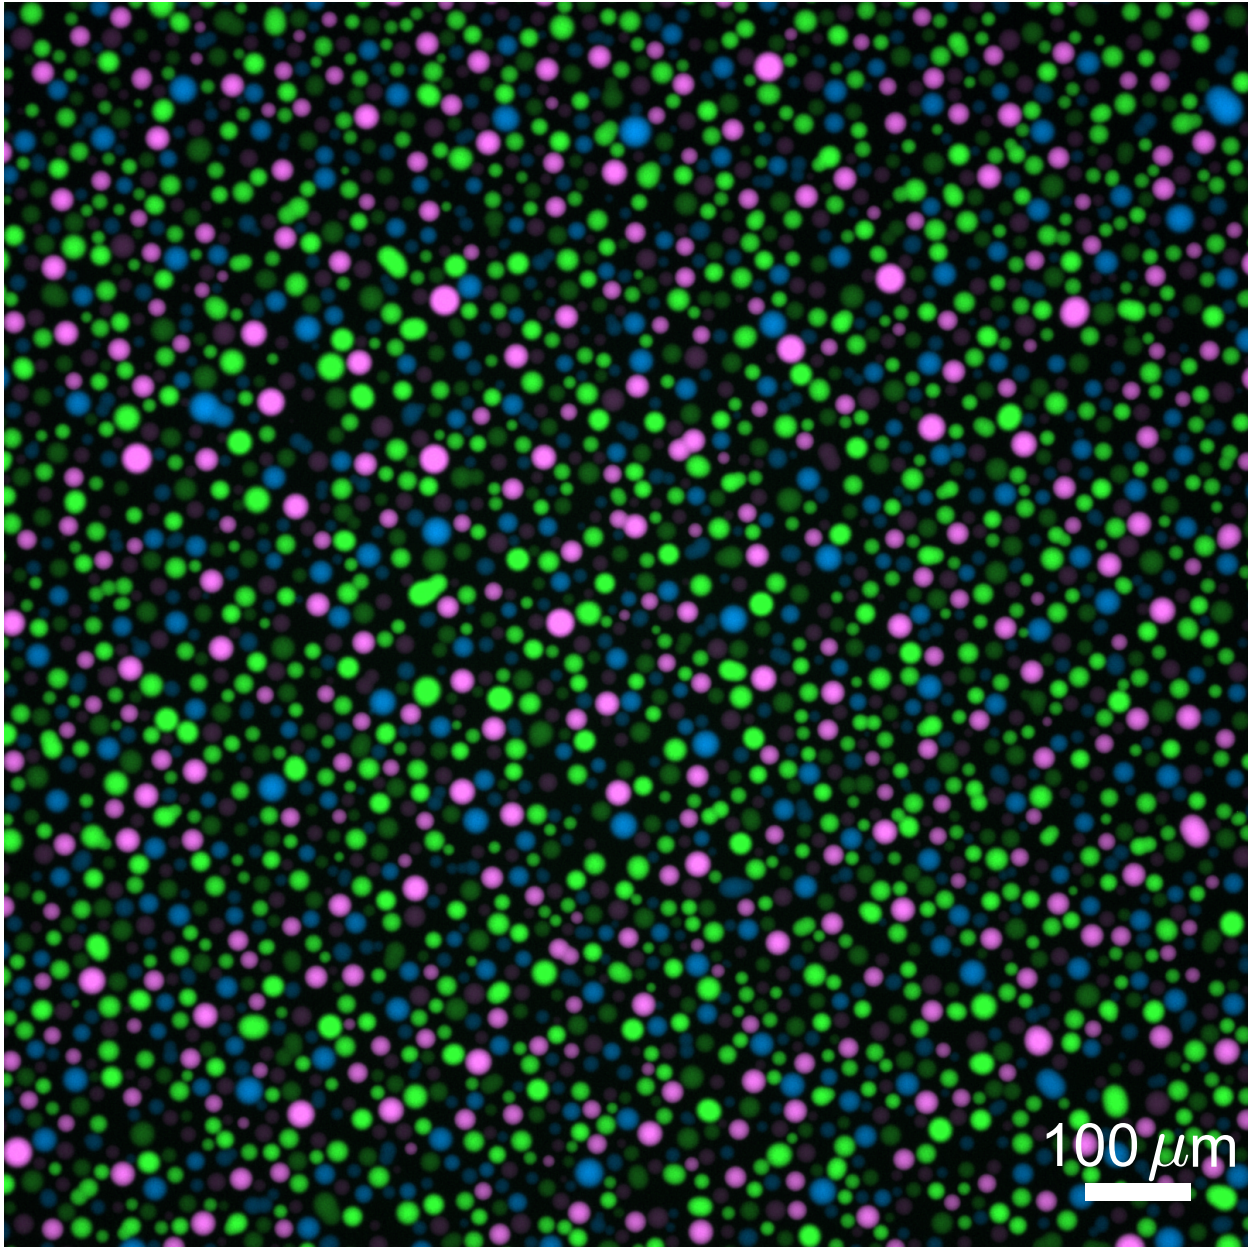

FIG. S10. Full size, three-color image of 7 droplet phases, associated with the cropped image corresponding to  $t = 16\text{h}$  after the slow temperature ramp in Fig. 4A of the main text.

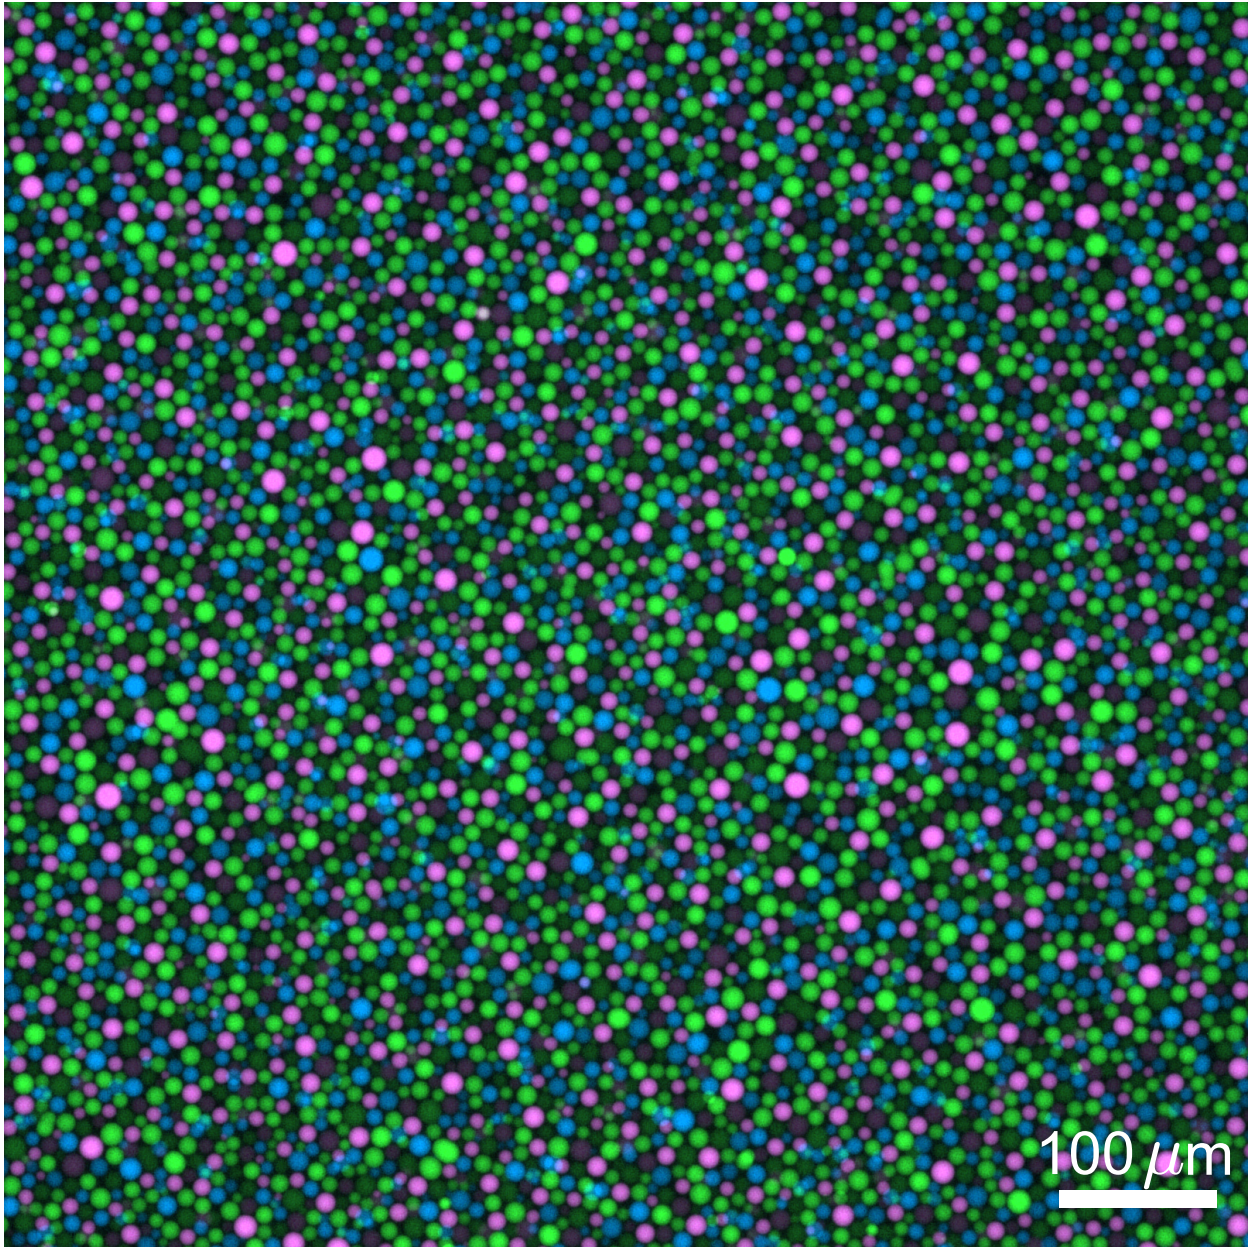

FIG. S11. Full size, three-color image of 7 droplet phases, associated with the cropped image corresponding to  $t = 16\text{h}$  after the rapid temperature quench in Fig. 4C of the main text.

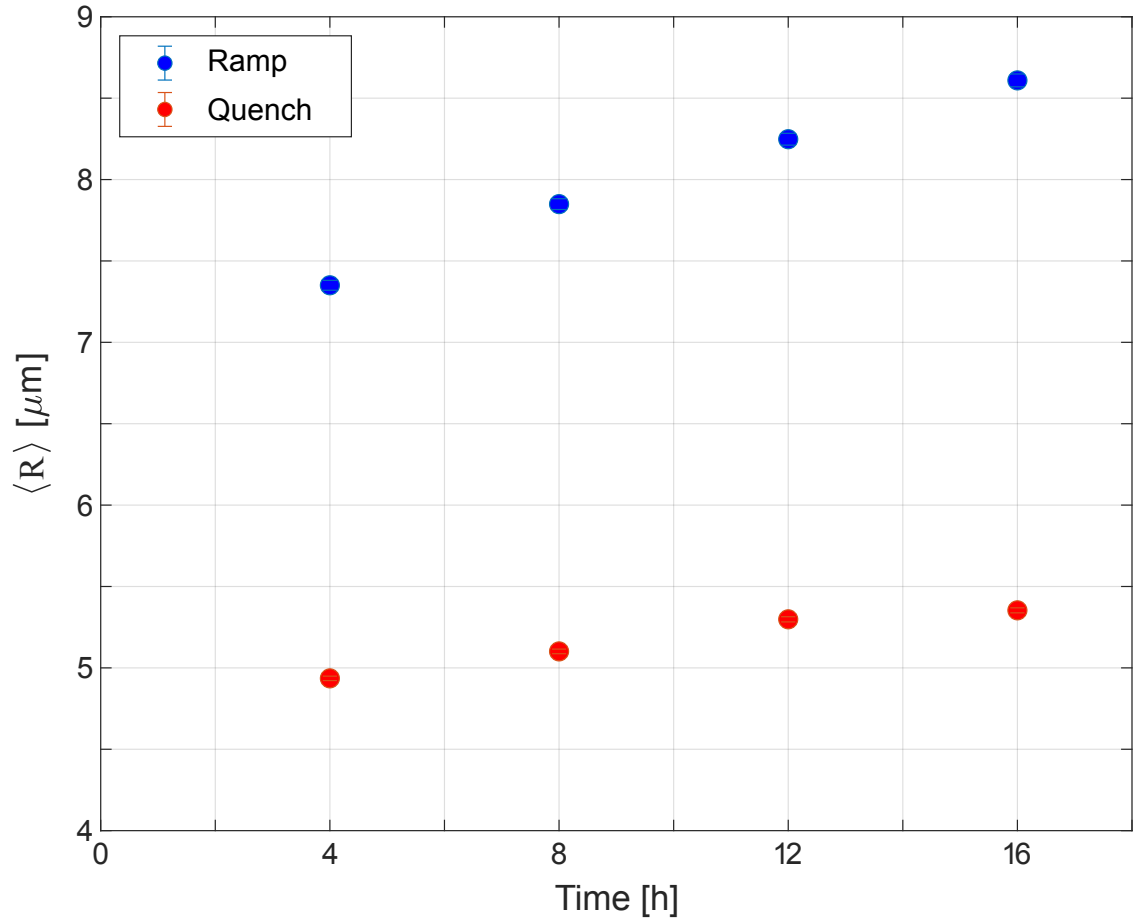

FIG. S12. Mean droplet radius grows more rapidly after the temperature ramp than after the quench (see also Fig. 4, 5). Error bars reflect the SEM.

- 
- [1] John SantaLucia Jr and Donald Hicks. The thermodynamics of DNA structural motifs. Annu. Rev. Biophys. Biomol. Struct., 33:415–440, 2004.
  - [2] Lorenzo Rovigatti, Francesca Bomboi, and Francesco Sciortino. Accurate phase diagram of tetravalent DNA nanostars. The Journal of Chemical Physics, 140(15):154903, 2014.
